# Supplementary material for: Scaled and Dynamic Optimizations of Nudged Elastic Bands
Source: arXiv:1906.10257 ancillary file (2019-06-24)
Supplement: Supplementary file 1 [file SupportingInformation.pdf]

# Supporting information for:
# Scaled and Dynamic Optimizations of Nudged Elastic Bands

Per Lindgren, Georg Kastlunger, and Andrew A. Peterson*

*School of Engineering, Brown University, Providence, Rhode Island, 02912, USA*

## CONTENTS

Dynamic relaxation of interior states 1

Scaling factor and smoothness of band 3

Computational details 4

References 4

## DYNAMIC RELAXATION OF INTERIOR STATES

We highlight examples of dynamic relaxations for the Tafel reaction on Au(111) with seven interior states. Figure 1 shows the converged band without (left) and with (right) climbing. For simplicity, the convergence criteria are scaled in multiples of $f_{\max}^{i_{\max}}$. The convergence criterion of each state is based upon the index of the state relative to the state with the highest potential energy,

$$f_{\max}^{i} = f_{\max}^{i_{\max}} \cdot (1 + |i_{\max} - i| \cdot \alpha_{\mathrm{s}}), \tag{1}$$

where the index $i$ loops over the interior states, $i_{\max}$ is the index of the interior state with the highest energy, $f_{\max}^{i_{\max}}$ is the tight convergence criterion given to the optimizer and $\alpha_{\mathrm{s}}$ is the scaling factor.

The dynamic implementation with $\alpha_{\mathrm{s}} = 1$ is shown in black and the default implementation in gray. Note that the highest image, $i_{\max}$, has essentially identical energy between the two methods; the energy difference is $\Delta E = 1 - 2$ meV. However, the low-energy regions of the PES differ in geometry and energy, since the dynamic implementation with scaled convergence criteria does not unnecessarily recalculate converged states.

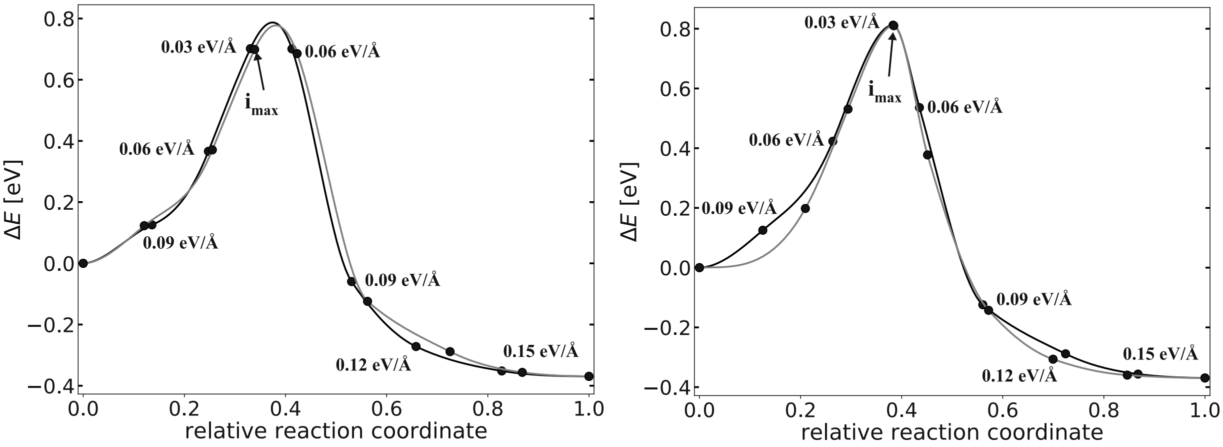


**FIG. 1:** Minimum energy pathway for the Tafel reaction of HER on Au(111) with $\alpha_{\mathrm{s}} = 1$. The convergence criteria are scaled in multiples of $f_{\max}^{i_{\max}}$. The left panel shows the band before climbing, and the right panel shows the converged band after climbing. The black and gray curves represent the dynamic implementation with $\alpha_{\mathrm{s}} = 1$ and the default implementation, respectively.

As noted in the main article, converged states can be recalculated if their neighboring states are optimized. This is shown in figure 2 for all states in the band without climbing. The first interior state converges after 57 optimization steps, but is perturbed out of convergence when the neighboring state changes its geometry. The movement of the neighboring state changes the spring force between the pair of images, causing the first state to be recalculated. For the sixth interior state, we observe two linear regions where the forces are constant. Here, the state *and* its neighbors are converged. Thus, the PES-derived forces and the spring forces between the state and its neighbors are constant.

Figure 3 shows the same analysis for the climbing-image implementation. Here, only states close to the saddle point are optimized, and most states are skipped during optimization. In this particular example, 85 out of 133 force calls were skipped.

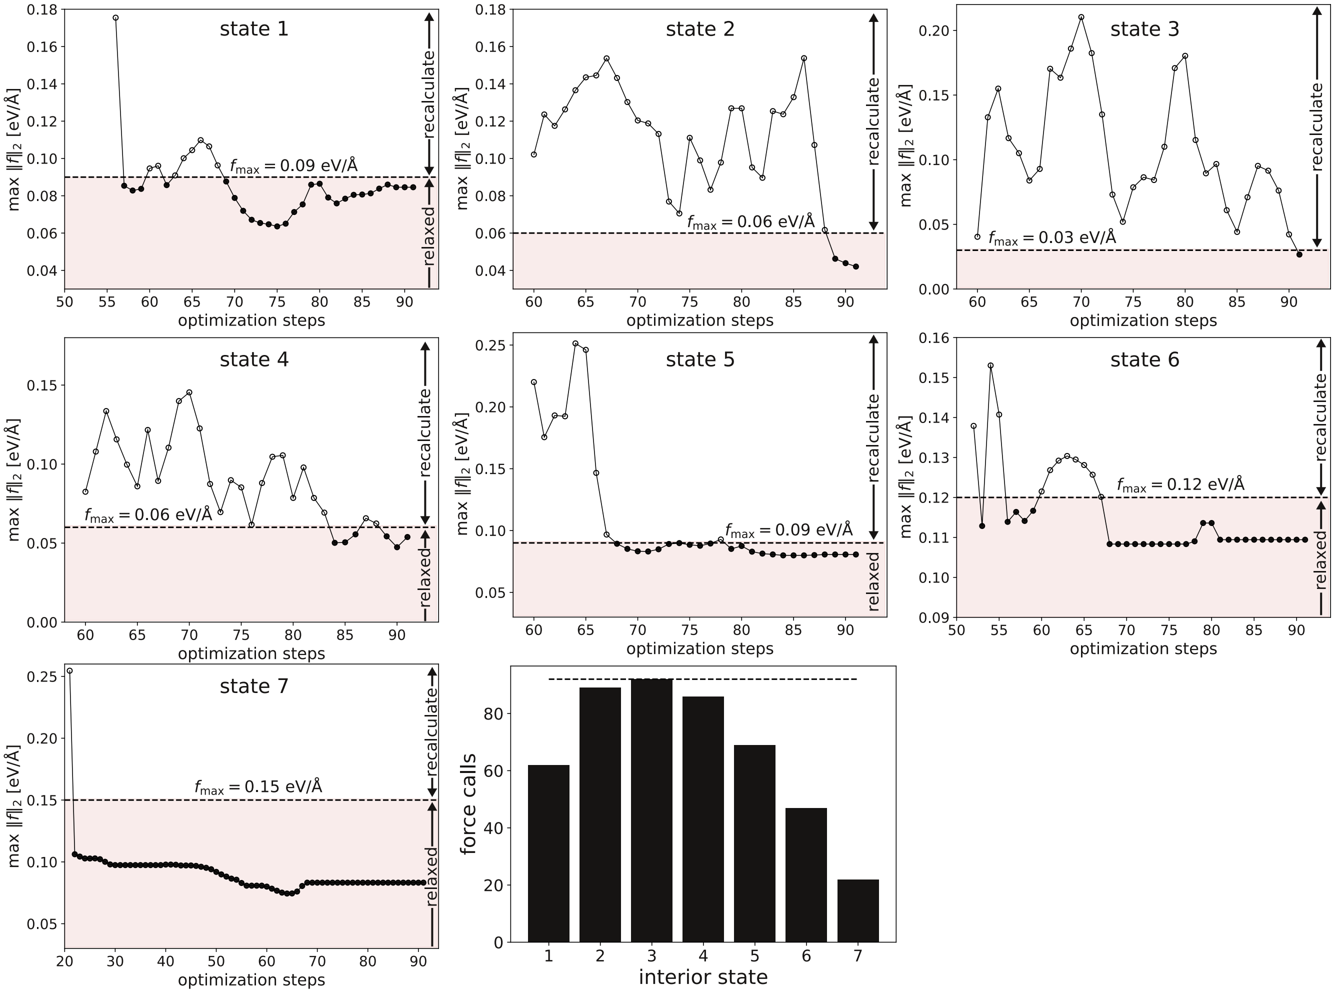


**FIG. 2:** Dynamic relaxation of interior states for the Tafel reaction of HER on Au(111) without climbing. Solid and open circles represent states below and above the convergence criterion, respectively. Note that geometry optimization of a neighboring state can perturb the forces of a converged state.

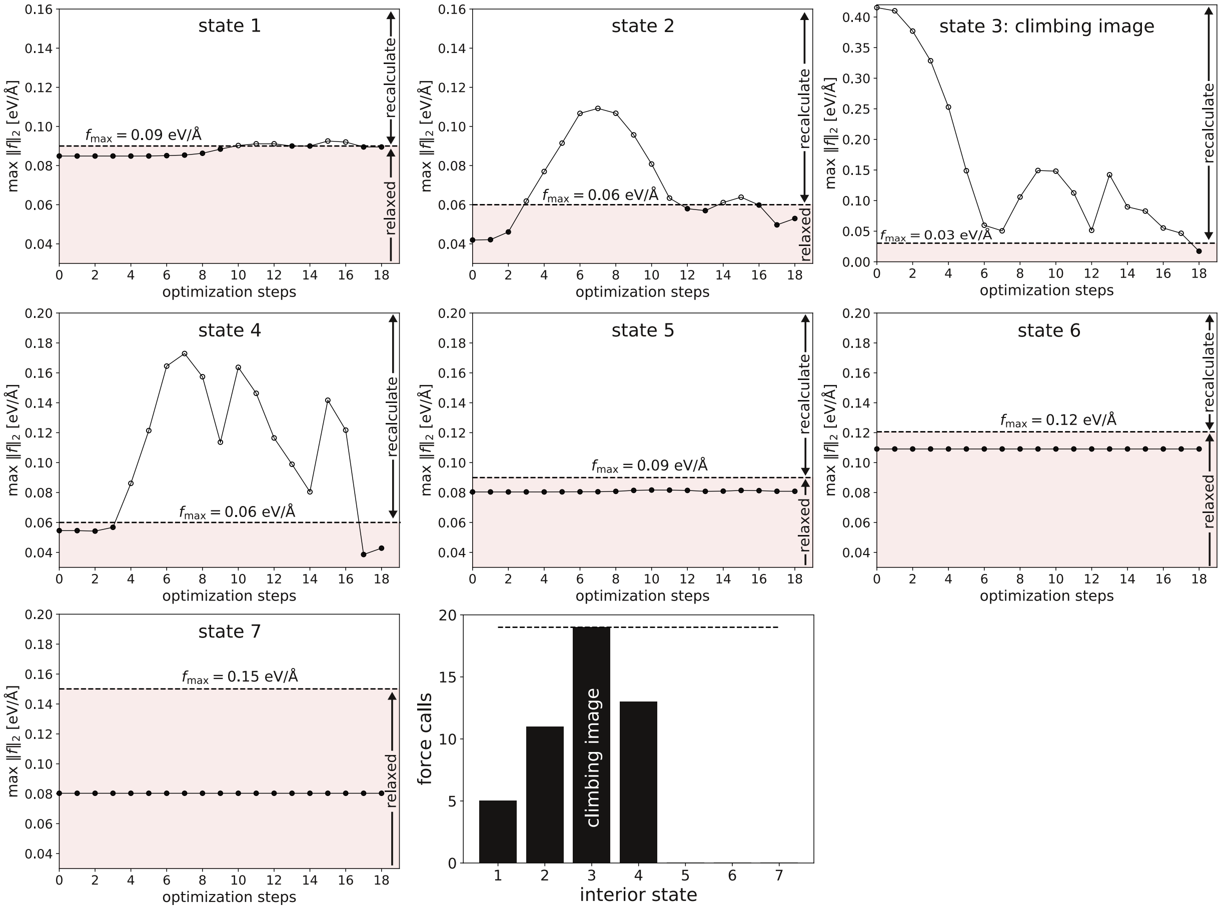


**FIG. 3:** Dynamic relaxation of interior states for the Tafel reaction of HER on Au(111) with climbing. Most states are skipped, and only the points close to the saddle point are optimized.

## SCALING FACTOR AND SMOOTHNESS OF BAND

As noted in the main article, the smoothness of the converged band depends upon the scaling factor; a steeper ramping of the convergence criteria decreases the number of force calls needed for convergence, but can also disrupt the pathway. Figure 4 shows the minimum energy pathways for three cases: the default implementation (black) and displacement scaling with $\alpha_s = 6$ and $\alpha_s = 20$. The number of force calls required to reach convergence ($f_{max} = 0.03$ eV/Å) is shown in the bar graph. The dynamic implementation with a relatively low scaling factor ($\alpha_s = 6$) decreases the number of force calls by 75% without disrupting the pathway of the band, *i.e.,* the pathway between the two stable states is smooth. However, the higher scaling factor ($\alpha_s = 20$) only introduces a modest decrease in number of force calls compared to $\alpha_s = 6$, but the pathway is significantly altered. We recommend using a low scaling factor, since it introduces a significant reduction in force calls while closely resembling the true minimum energy pathway.

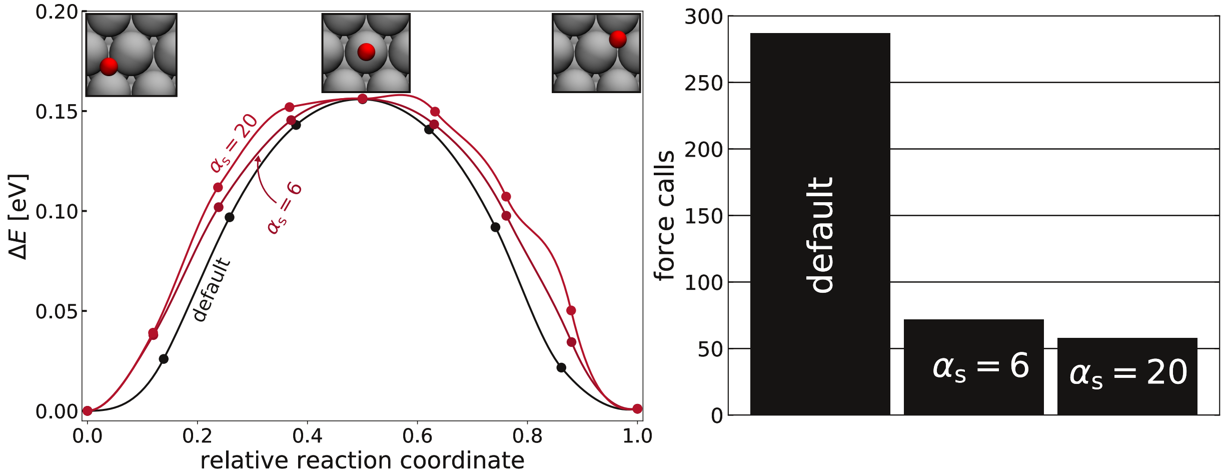


**FIG. 4:** Minimum energy pathways of oxygen diffusion on Pt(111) for the default and displacement scaling NEB implementations. A relatively low scaling factor significantly decreases the number of force calls while maintaining a smooth band between the two endstates.

## COMPUTATIONAL DETAILS

All calculations were carried out in the Atomistic Simulation Environment (ASE) [1]. The Tafel reactions were calculated with the grid-based projector augmented wave method (GPAW) [2, 3] and the Perdew-Burke-Ernzerhof (PBE) exchange-correlation functional [4]. The bottom layer of the 3×3×3 Au(111) surface was constrained at the bulk-optimized lattice constant (4.18 Å), and a dipole-correction [5] was applied along the direction perpendicular to the surface. The system was sampled on a 4×4×1 **k**-point mesh, and all local minima and saddle points were optimized until the forces acting on all unconstrained atoms were below 0.03 eV/Å. Saddle points were confirmed with normal mode analyses; one imaginary frequency—representing the reaction coordinate—was observed for each system.

The Heyrovsky reaction was calculated with the Solvated Jellium (SJ) method [6]. This electronically grand canonical code includes a compensation charge immersed in an implicit solvent [7]. The implicit solvent introduces a spatially dependent dielectric constant in the unit cell. The charge neutral Jellium slab includes explicit charge and a counter charge of equal magnitude but opposite sign. The former is optimized in the self-consistent field (SCF) cycle of DFT, while the latter is spatially constrained in the implicit solvent region. The Au(111) was modeled as a 3×2×3 surface with the PBE exchange-correlation functional and a 4×6×1 **k**-point mesh. The FIRE [8] optimizer was used during climbing.

* andrew_peterson@brown.edu

[1] A. H. Larsen, J. J. Mortensen, J. Blomqvist, I. E. Castelli, R. Christensen, M. Dułak, J. Friis, M. N. Groves, B. Hammer, C. Hargus, E. D. Hermes, P. C. Jennings, P. B. Jensen, J. Kermode, J. R. Kitchin, E. L. Kolsbjerg, J. Kubal, K. Kaasbjerg, S. Lysgaard, J. B. Maronsson, T. Maxson, T. Olsen, L. Pastewka, A. Peterson, C. Rostgaard, J. Schiøtz, O. Schütt, M. Strange, K. S. Thygesen, T. Vegge, L. Vilhelmsen, M. Walter, Z. Zeng, and K. W. Jacobsen, Journal of Physics: Condensed Matter **29**, 273002 (2017).
[2] J. J. Mortensen, L. B. Hansen, and K. W. Jacobsen, Physical Review B **71**, 35109 (2005).
[3] J. Enkovaara, C. Rostgaard, J. J. Mortensen, J. Chen, M. Dułak, L. Ferrighi, J. Gavnholt, C. Glinsvad, V. Haikola, H. A. Hansen, H. H. Kristoffersen, M. Kuisma, A. H. Larsen, L. Lehtovaara, M. Ljungberg, O. Lopez-Acevedo, P. G. Moses, J. Ojanen, T. Olsen, V. Petzold, N. A. Romero, J. Stausholm-Møller, M. Strange, G. A. Tritsaris, M. Vanin, M. Walter, B. Hammer, H. Häkkinen, G. K. H. Madsen, R. M. Nieminen, J. K. Nørskov, M. Puska, T. T. Rantala, J. Schiøtz, K. S. Thygesen, and K. W. Jacobsen, Journal of Physics: Condensed Matter **22**, 253202 (2010).
[4] J. P. Perdew, K. Burke, and M. Ernzerhof, Physical Review Letters **77**, 3865 (1996).
[5] L. Bengtsson, Physical Review B **59**, 12301 (1999).
[6] G. Kastlunger, P. Lindgren, and A. A. Peterson, The Journal of Physical Chemistry C **122**, 12771 (2018).
[7] A. Held and M. Walter, The Journal of Chemical Physics **141**, 174108 (2014).
[8] E. Bitzek, P. Koskinen, F. Gähler, M. Moseler, and P. Gumbsch, Physical Review Letters **97**, 170201 (2006).
